# Supplementary material for: CsrA and its regulators control the time-point of ColicinE2 release in Escherichia coli
Source: arXiv:1805.02068 source file (2018-05-05)
Supplement: Supplementary file 1 [file arxiv_SI.pdf]

**Supplementary information for**

# Title: CsrA and its regulators control the time-point of ColicinE2 release in *Escherichia coli*

**Alexandra Götz, Matthias Lechner, Andreas Mader, Benedikt von Bronk, Erwin Frey and Madeleine Opitz**

## Supplementary Information (experimental)

*Accumulation of single-stranded DNA (ssDNA)*

Recently, Morales *et al.*(1), detected the accumulation of ssDNA in *Escherichia coli* cells carrying any one of the plasmids pColE3-CA38, pColE9 and pColE5. This ssDNA originates from rolling-circle replication(1, 2). This type of replication enables an autonomous plasmid to replicate independently of the bacterial cell cycle and cell division(3). The replicons of the plasmids pColE2-P9 and pColE3-CA38 are closely related(4), indicating that asymmetric rolling-circle replication(5) of the pColE2-P9 plasmid (**Fig S5a**) could also lead to ssDNA accumulation, as shown in **Fig 3 and Fig S5b**. Furthermore, sequencing of pColE2-P9 and an analysis of its homology with pColE3-CA38 (**Table S1**) confirms the close relationship between the two plasmids. The Rep protein binds to the ColE2 *ori* to initiate rolling-circle replication(3), leading to ssDNA synthesis(2). The concentration of the Rep protein is held constant by the action of an anti-sense sRNA (the *inkA* gene product) that binds to the 5'-untranslated region of the mRNA encoding the Rep protein(6).

Please note that the reporter plasmid pMO3(7) used in this study is a derivative of pBAD24. Its replication mode(8) differs from that of pColE2-P9 and does not lead to the accumulation of ssDNA (**Fig 3**)(1).

*Supplementary Methods*

In the following, additional information relating to the construction of the specific mutant strains used in this study is given, together with a description of RNA and ssDNA oligos used for CsrA binding studies. **Table S2** provides an overview of all (mutant) strains used in this study. **Table S3** summarizes all primers used, including those employed in the construction of the mutant strains listed in **Table S4** and in sequencing of pColE2-P9. **Table S4** lists the base-pair changes introduced into the plasmid pMO3 that resulted in plasmids pMO4, pMO5, pMO6, pMO7, as well as the sequences of RNA and ssDNA oligos used for CsrA-binding studies as described in the **Methods** section of the main text.

**Supplementary Tables**

**Table S1: Sequence homology of genes present on the plasmids pColE2-P9 and pColE3-CA38.** Numbers in red indicate that the gene extends past the base-pair designated as position 1.

| Gene | Sequence position on pColicinE2-P9 | Sequence position on pColE3-CA38 | Homology E2/E3 |
|---|---|---|---|
| *rep* | 3073-3792 | 3344-4258 | 97% |
| *ssi* | 4084-4159 | 4376-4451 | 100% |
| *mob* | 4182-4456 | 4475-4750 | 98% |
| *tra* | 4636-6757,1-98 | 4929-7118,1-30 | 97% |
| *incA* | 2943-3057 | 3214-3328 | 100% |
| colE2/E3 ori | 3966-3997 | 4257-4289 | 94% |

**Table S2: Bacterial strains used in this study**

| Bacterial strain | Strain description | Genetic modification/information | Reference |
|---|---|---|---|
| BZB 1011 | | | (9) |
| $C_{WT}$ (BZB 1011 E2C) | | Carries pColE2-P9 | (9) |
| $C_{REP1}$ (EMO3-C) | BZB 1011 E2C pMO3 | Carries pColE2-P9 and the reporter plasmid pMO3 | (7) |
| $S_{REP1}$ (EMO3-S) | BZB 1011 pMO3 | Same as EMO3-C without the Colicin E2 plasmid | (7) |
| LexA1 | BZB 1011 pMO4 Derivative of $S_{REP1}$ | LexA binding sequence altered on pMO3 to achieve stronger LexA binding, resulting in pMO4 | This study |
| LexA2 | BZB 1011 pMO5 Derivative of $S_{REP1}$ | LexA binding sequence altered on pMO3 to achieve weaker LexA binding, resulting in pMO5 | This study |
| CsrA1 | BZB 1011 pMO6 Derivative of $S_{REP1}$ | CsrA binding sequence on pMO3 altered to achieve stronger CsrA binding, resulting in pMO6 | This study |
| CsrA2 | BZB 1011 pMO7 Derivative of $S_{REP1}$ | CsrA binding sequence on pMO3 altered to achieve weaker CsrA binding, resulting in pMO7 | This study |
| CsrB (EMO3::CsrB) | BZB 1011 CsrB::Kan pMO3 Derivative of $S_{REP1}$ | CsrB::Kan, in-frame replacement of CsrB by a kanamycin resistance | This study |
| CsrC (EMO3::CsrC) | BZB 1011 CsrC::Kan pMO3 Derivative of $S_{REP1}$ | CsrC::Kan, in-frame replacement of CsrC with a kanamycin resistance | This study |
| CsrBC<br><br>(EMO3::CsrBC) | BZB 1011 CsrB::Cam CsrC::Kan pMO3 Derivative of $S_{REP1}$ | CsrC::Kan, CsrB::Cam, in-frame replacement of CsrC by a kanamycin resistance and of CsrB by a chloramphenicol resistance cassette | This study |
| $C_{REP2}$ | BZB 1011 E2C pMO8 | Same as $C_{REP1}$, only the origin of replication on pMO3 has been changed to p15A to achieve a lower copy number of 13 copies per cell - pMO8 | This study |
| $S_{REP2}$ | BZB 1011 pMO8 | Same as $S_{REP1}$, only the origin of replication on pMO3 has been changed to p15A to achieve a lower copy number of 13 copies per cell -> pMO8 | This study |

**Table S3: Primers used in this study.** Primers P1-P12 were used for construction of the mutant strains listed in **Table S2**. Primers P13-P24 were used for sequencing pColE2-P9. Primer pairs P25/P26 and P27/28 were used to create the low copy plasmid pMO8.

| **Name** | **Sequence** | **Purpose** |
|---|---|---|
| P1 | 5´- GACGGGTACTTTTTGTACTGTACATAAAACCAGTGG - 3´ | LexA1 [fwd] cloning |
| P2 | 5´- CCACTGGTTTTATGTACAGTACAAAAAGTACCCGTC- 3´ | LexA1 [rev] cloning |
| P3 | 5´- GACGGGTACTTTTTGATCCCTACATAAAACCAGTGG- 3´ | LexA2 [fwd] cloning |
| P4 | 5´- CCACTGGTTTTATGTAGGGATCAAAAAGTACCCGTC- 3´ | LexA2 [rev] cloning |
| P5 | 5´- GGCATTCTTTCACATTAAGGAGTCGTTATG - 3´ | CsrA1 [fwd] cloning |
| P6 | 5´- CATAACGACTCCTTAATGTGAAAGAATGCC- 3´ | CsrA1 [rev] cloning |
| P7 | 5´- GCATTCTTTCACAACAAGGATGTGTTATGAAAAAAATAACCGG-3´ | CsrA2 [fwd] cloning |
| P8 | 5´- CCGGTTATTTTTTTCATAACACATCCTTGTTGTGAAAGAATGC- 3´ | CsrA2 [rev] cloning |
| P9 | 5´GTGGTCATAAAGCAACCTCAATAAGAAAAACTGCCGCGAA GGATAGCAGG AATTAACCCTCACTAAAGGGCG 3´ | ΔCsrB [fwd] cloning |
| P10 | 5´TTGTCTGTAAGCGCCTTGTAAGACTTCGCGAAAAAGACGATTCTATCT TCTAATACGACTCACTATAGGGCTC 3´ | ΔCsrB [rev] cloning |
| P11 | 5´ ACTGATGGCG GTTGATTGTT TGTTTAAAGCAAAGGCGTAA AGTAGCACCCAATTAACCCTCACTAAAGGGCG 3´ | ΔCsrC [fwd] cloning |
| P12 | 5´GCCGTTTTATTCAGTATAGATTTGCGGCGGAATCTAACAGAAAGCAA GCATAATACGACTCACTATAGGGCTC 3´ | ΔCsrC [rev] cloning |
| | | |
| P13 | 5´- ACCGTATCTCCGTCATCAAC -3´ | ColE2-1 [fwd] sequencing |
| P14 | 5´- CTTCCTGTGAGAACTGC -3´ | ColE2-2 [fwd] sequencing |
| P15 | 5´- GTAGCGAGCGAATGAG -3´ | ColE2-3 [fwd] sequencing |
| P16 | 5´- CATGATTGCCGATGTGG -3´ | ColE2-4 [fwd] sequencing |
| P17 | 5´- GTGGAATACGTGGATTGC -3´ | ColE2-5 [fwd] sequencing |
| P18 | 5´- GGAGAAGCTATAAACCATG -3´ | ColE2-6 [fwd] sequencing |
| P19 | 5´- TCTGCTCATGTTTGACAGCTT -3´ | ColE2-7 [fwd] sequencing |
| P20 | 5´- CTCTGTTCGCATGGTCAG -3´ | ColE2-8 [rev] sequencing |
| P21 | 5´- CACGTTCGATGTCGTTC -3´ | ColE2-9 [rev] sequencing |
| P22 | 5´- GAATACATTCTCACACGCTC -3´ | ColE2-10 [rev] sequencing |
| P23 | 5´- CGTTGTTGTTGCCTGTG -3´ | ColE2-11 [rev] sequencing |
| P24 | 5´- TCATCCGCCAAAACAGCC -3´ | ColE2-12 [rev] sequencing |
| | | |
| P25 | 5´- ATTAAGTCGACGAAGATCCTTTGATCTTTTC -3´ | pMO3_noORI SalI [rev] Cloning pMO3 vector without ORI |
| P26 | 5´- ATTAAGCATGCAACGCCAGCAACGC -3´ | pMO3_noORI SphI[fwd] Cloning pMO3 vector without ORI |
| P27 | 5´- ATTAAGTCGACTTGAGATCGTTTTGG -3´ | p15A ORI SalI [rev] cloning |
| P28 | 5´- ATTAAGCATGCTTTCCATAGGCTCCG -3´ | p15A ORI SphI [fwd] cloning |

**Table S4. Sequences of genetic elements.** The first three rows depict sequence changes in the LexA binding site (two overlapping LexA binding SOS boxes) on the pMO3 reporter plasmid, leading to altered LexA binding (pMO4, pMO5). The following three rows show the changes made in the CsrA binding site within the second mRNA loop (which also includes the ribosome binding site of the *cel* gene and the GGA motif recognized by CsrA) that potentiate (pMO6) or weaken (pMO7) CsrA binding (**Fig 2d**). The following three rows list the sequences of RNA oligos used for CsrA binding studies (**Methods, Fig 2d**) and include the alterations in the CsrA binding site mentioned above. The last three rows give the sequences of the 89-bp ssDNA oligos used to study binding of CsrA to ssDNA by gel shift analysis (**Methods**). Bases highlighted in *green* correspond to sequence changes. Bases shown in boldface highlight the GGA motif required for CsrA binding as present within the second mRNA (plasmid), RNA oligo or ssDNA oligo loop. We confirmed the appropriate formation of secondary structures of these oligos using Mfold(10) (**Methods**).

| Name | Sequence | Description |
|---|---|---|
| pMO3 | 5‘-TTGATCTGTACATAAAACCAGTGGTTTTATGTACAGTATTAA-3‘ | LexA binding site |
| pMO4 | 5‘-TTGTACTGTACATAAAACCAGTGGTTTTATGTACAGTATTAA-3‘ | LexA binding site |
| pMO5 | 5‘-TTGATCCCTACATAAAACCAGTGGTTTTATGTACAGTATTAA-3‘ | LexA binding site |
| pMO3 | 5' - CACAACAA**GGA**GTCGTTATG - 3' | CsrA binding site second loop |
| pMO6 | 5' - CACAACAA**GGA**TGTGTTATG - 3' | CsrA binding site second loop |
| pMO7 | 5' - CACATTAA**GGA**GTCGTTATG - 3' | CsrA binding site second loop |
| RNA Oligo equivalent to sequence of pMO3 | 5‘-Cy5- AUUUAAACAGGGCUGAAAUAUGAAUGCCGGUUGUUUAU **GGA**UGAAUGGCUGGCAUUCUUUCACAACAA**GGA**GUCGUUAUGA AAAAAUA -3‘ | RNA Oligo with both CsrA binding sites (GGA) |
| RNA Oligo equivalent to sequence of pMO6 | 5‘-Cy5- AUUUAAACAGGGCUGAAAUAUGAAUGCCGGUUGUUUAU **GGA**UGAAUGGCUGGCAUUCUUUCACAACAA**GGA**UGUGUUAUGA AAAAAUA -3‘ | RNA Oligo with both CsrA binding sites (GGA) |
| RNA Oligo equivalent to sequence of pMO7 | 5‘-Cy5- AUUUAAACAGGGCUGAAAUAUGAAUGCCGGUUGUUUAU **GGA**UGAAUGGCUGGCAUUCUUUCACAUUAA**GGA**GUCGUUAUG AAAAAAUA -3‘ | RNA Oligo with both CsrA binding sites (GGA) |
| ssDNA Oligo equivalent to sequence of pMO3 | 5‘-Cy5- ATTTAAACAGGGCTGAAATATGAATGCCGGTTGTTTAT **GGA**TGAATGGCTGGCATTCTTTCACAACAA**GGA**GTCGTTATG AAAAAAATA - 3‘ | ssDNA Oligo with both CsrA binding sites (GGA) |
| ssDNA Oligo equivalent to sequence of pMO6 | 5‘-Cy5-ATTTAAACAGGGCTGAAATATGAATGCCGGTTGTTTAT **GGA**TGAATGGCTGGCATTCTTTCACAACAA**GGA**TGTGTTATG AAAAAATA -3‘ | ssDNA Oligo with both CsrA binding sites (GGA) |
| ssDNA Oligo equivalent to sequence of pMO7 | 5‘-Cy5- ATTTAAACAGGGCTGAAATATGAATGCCGGTTGTTTAT GGATGAATGGCTGGCATTCTTTCACATTAA**GGA**GTCGTTATG AAAAAATA -3‘ | ssDNA Oligo with both CsrA binding sites (GGA) |

## Supplementary Figures

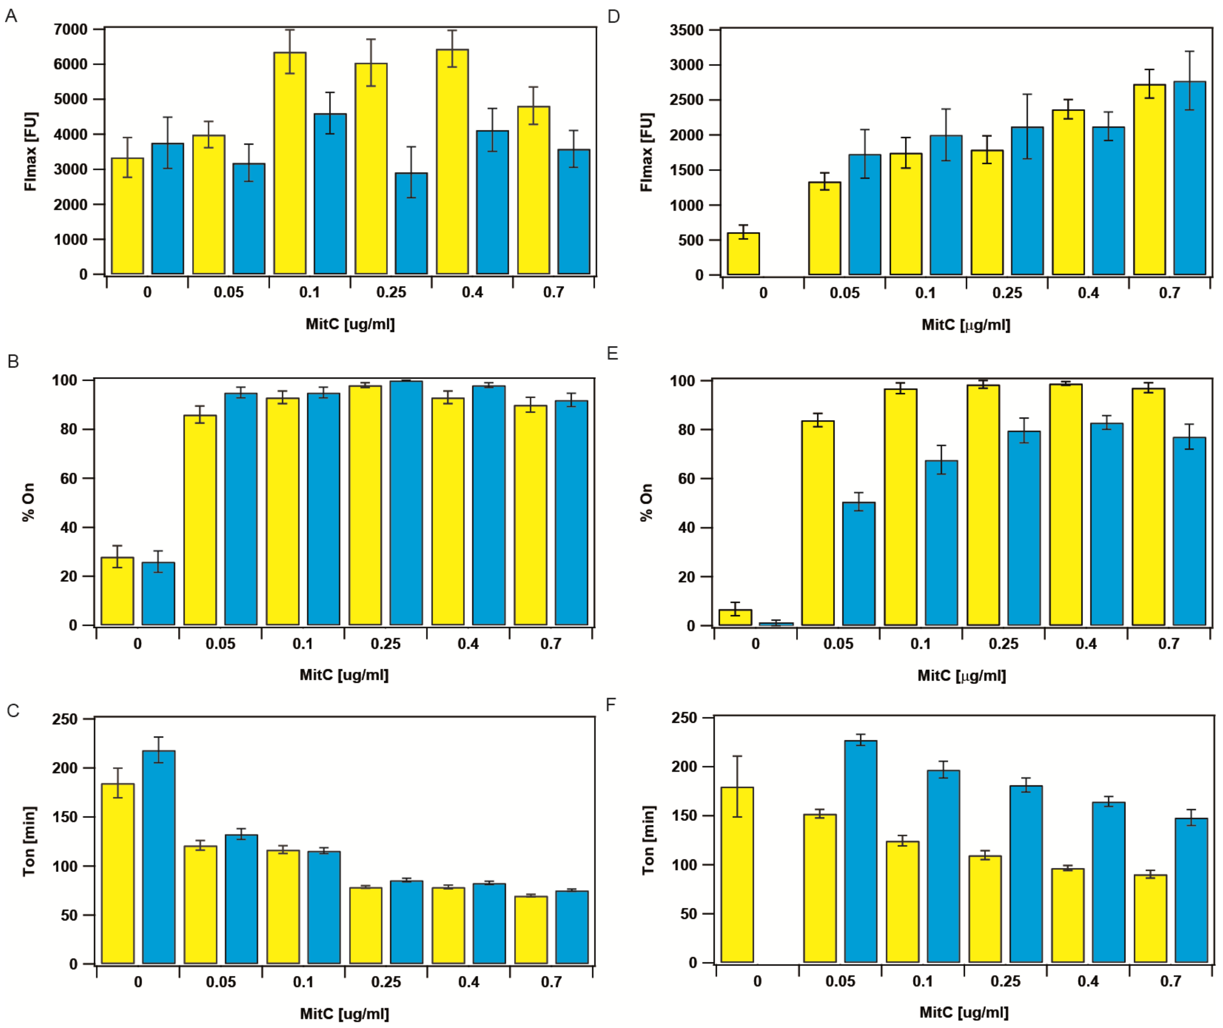


**Fig S1: Dependence of the maximal fluorescence intensity, cumulative fraction and time-point of expression start of cells expressing the ColicinE2 operon in the $C_{REP1}$ and $S_{REP1}$ strains on the MitC concentration.** Yellow: *cea* gene expression (colicin production), blue: *cel* gene expression (colicin release). Data shown here represent average values obtained from single-cell time-lapse microscopy experiments. A-C) $C_{REP1}$, D-F) $S_{REP1}$, A,D) Maximal fluorescence intensity of the cells that express the ColicinE2 operon. B,E) Cumulative fraction of cells expressing the ColicinE2 operon. C,F) Onset ($t_{ON}$) of *cea* and *cel* gene expression.

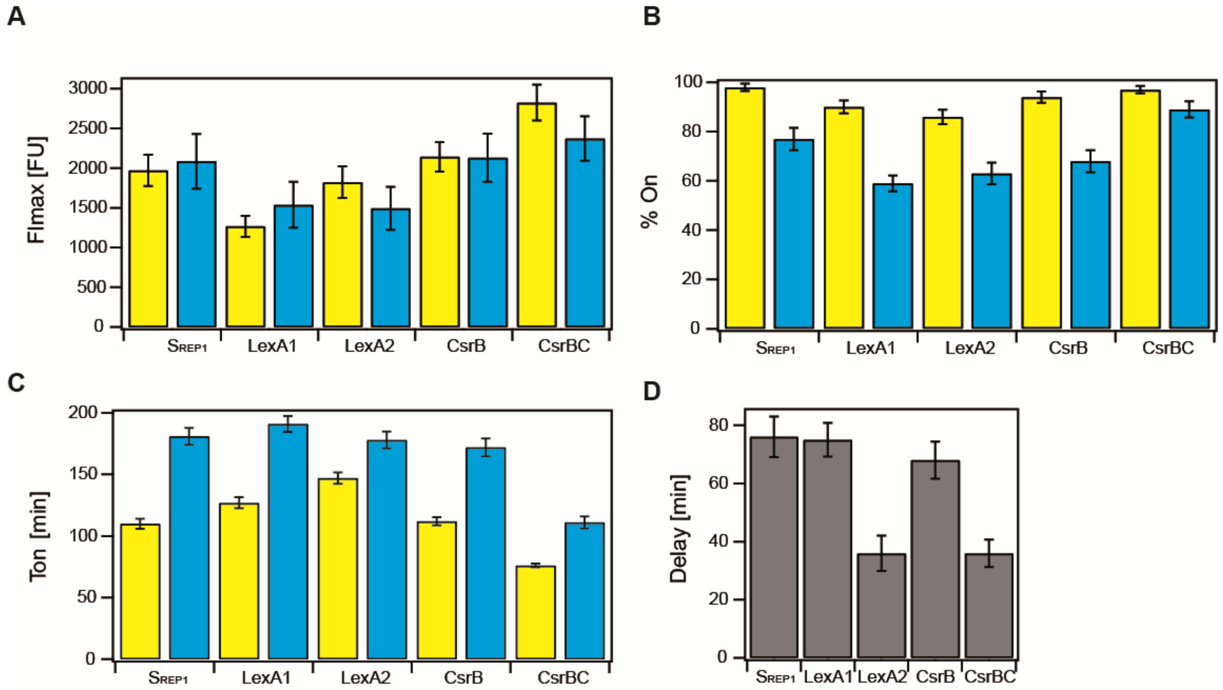


**Fig S2: Impact of alteration of the LexA binding site or absence of sRNAs on ColicinE2 expression in $S_{REP1}$ cells. A-C)** Yellow: *cea* gene expression (colicin production), blue: *cel* gene expression (colicin release). **A)** Mean maximal expression of the colicin operon (relative to the $\mathbf{S_{REP1}}$ strain) in mutant reporter strains bearing altered LexA binding sites (LexA1 and LexA2, **SI, Methods**), or lacking the sRNA CsrB (CsrB), or missing both sRNAs CsrB and CsrC (CsrCB). **B)** Cumulative fraction of cells expressing the colicin operon. **C)** $T_{ON}$ times for *cea* and *cel* gene expression. **D)** Delay between *cea* and *cel* gene expression.

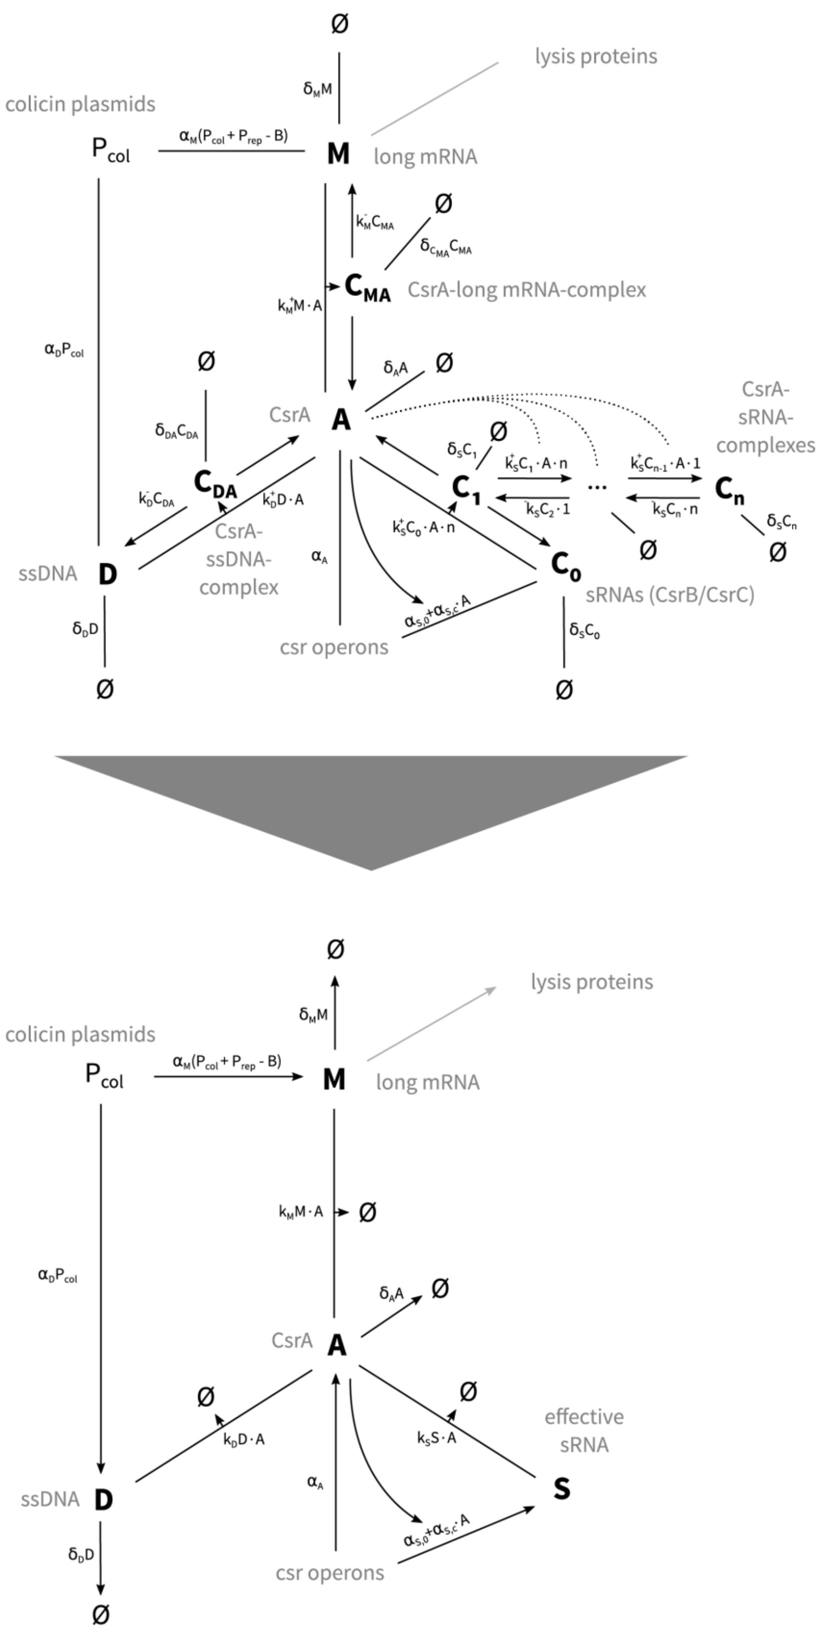


**Fig S3: Biochemical network involved in the post-transcriptional regulation of ColicinE2.** The top part shows the complete network, involving all interactions and components considered in this work. This complex description of the network can be reduced to the set of effective interactions shown in the lower panel. The derivation of these effective descriptions is given in section 2 of the theory part of the **SI.**

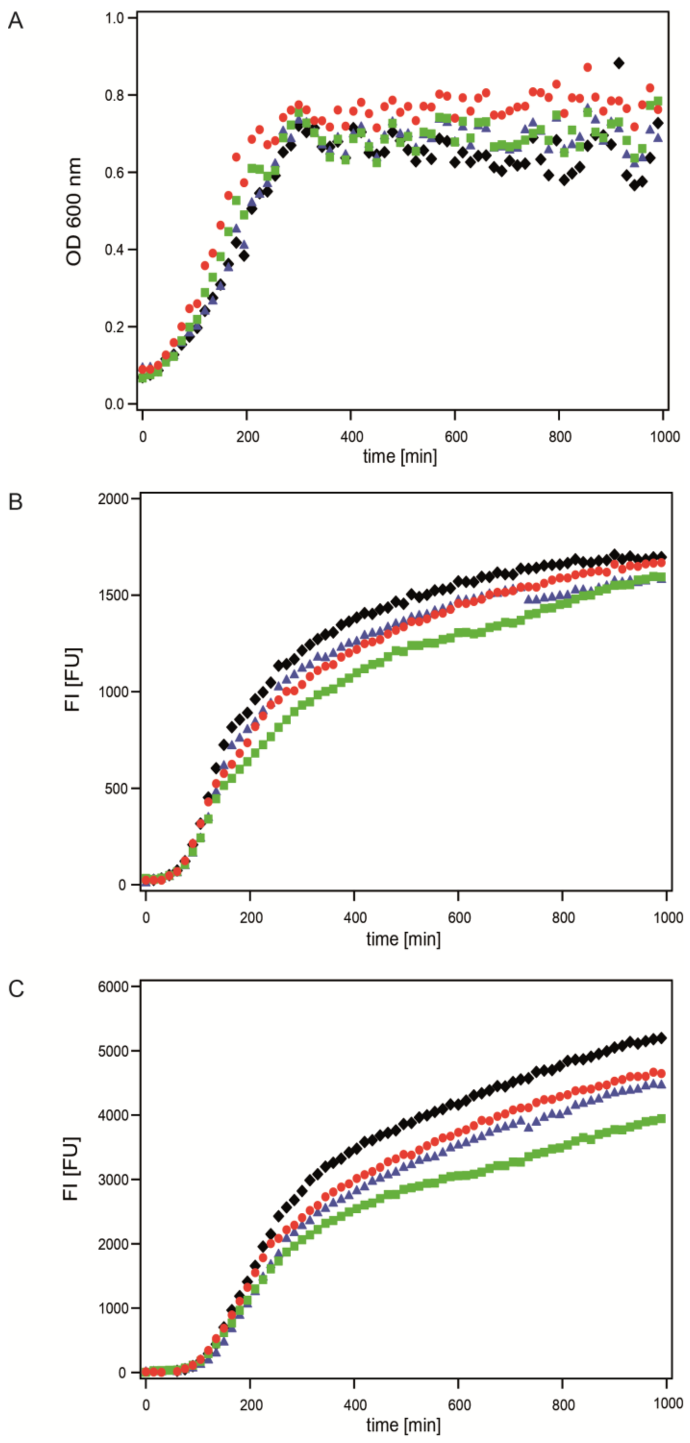


**Fig S4: Effect of sRNA knock-out on Colicin E2 expression in long-term experiments (0.25 µg/ml MitC).** To determine the importance of sRNA regulation for ColicinE2 expression over a longer period, plate-reader experiments were performed as described in **Methods**. **A)** Absorbance, **B)** Fluorescence intensity of cells expressing *cea* (YFP, colicin production), **C)** Fluorescence intensity of cells expressing *cel* (CFP, colicin release). Red: $S_{REP1}$ strain, Blue: CsrC single sRNA knock-out, Green: CsrB single sRNA knock-out, Black: CsrB/C double sRNA knock-out.

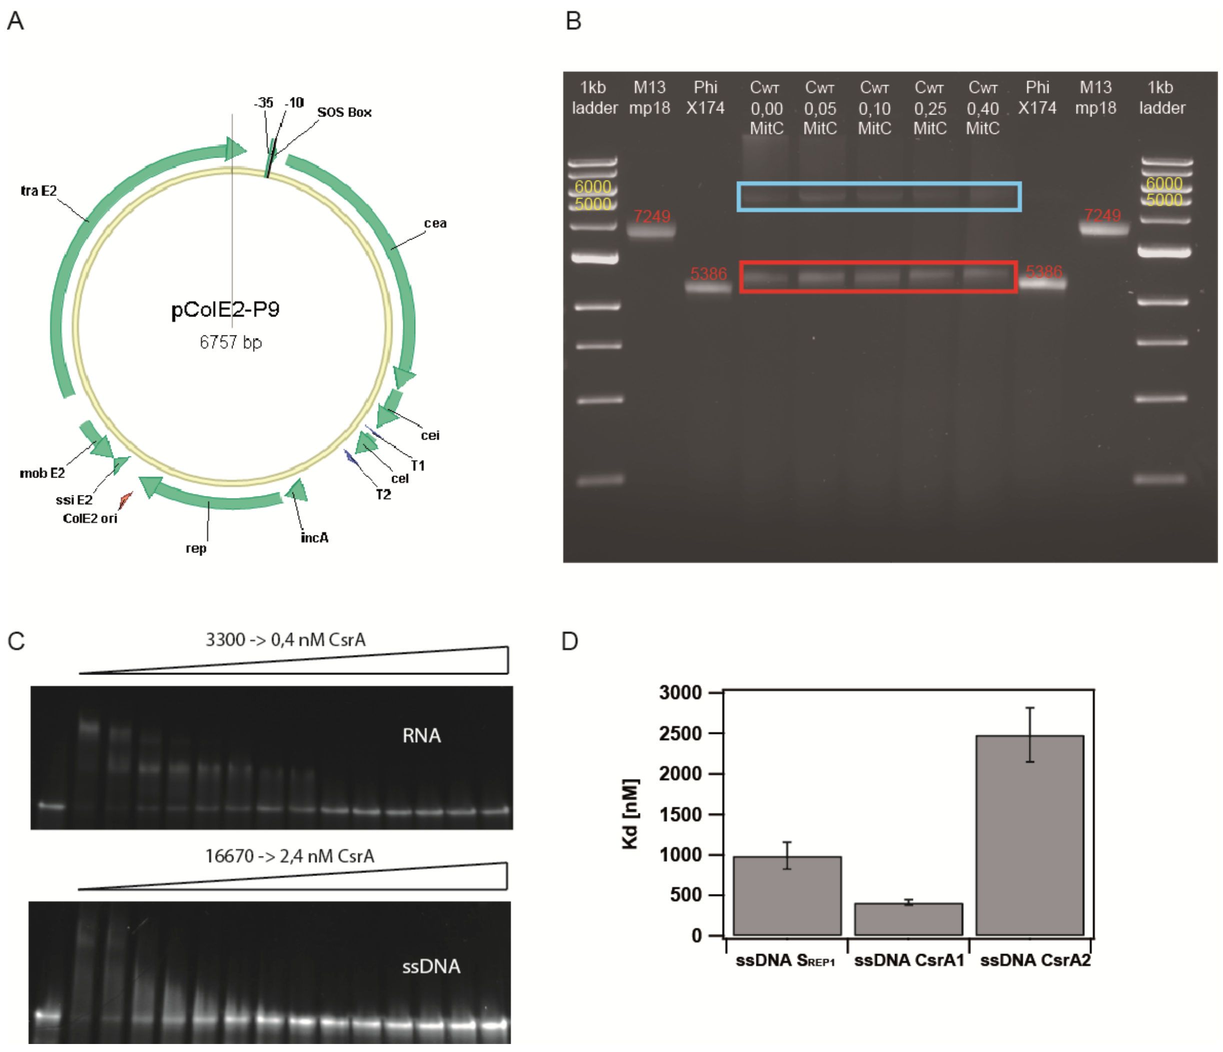


**Fig S5: ssDNA accumulation in bacteria carrying pColE2-P9 and binding of CsrA to ssDNA**. **A)** Map of pColE2-P9. The plasmid map was created using Vector NTI Expression Version 1.6.0. The plasmid sequence can be accessed via Genbank accession number KY348421. **B)** Accumulation of ssDNA in $C_{WT}$ is independent of the presence of MitC. Agarose gel of plasmid and ssDNAs extracted from $C_{WT.}$ Lanes 1-3 and 9-11 were loaded with the indicated markers: 1-kb ladder, 7249-bp ssDNA ring (M13mp18), and 5386-bp ssDNA ring (PhiX174). Lane 4-8: uncleaved $C_{WT}$ DNA showing the 6800-bp pColE2-P9 dsDNA (blue) and ssDNA (red) at different concentrations of the SOS inducing agent MitC. The staining substance ETBR binds optimal to dsDNA and only to ssDNA if secondary structures (ds part of ssDNA) are present. Hence, binding of ETBR to ssDNA is much lower than to dsDNA. Consequently, the brighter ssDNA bands reflect the high amount of ssDNA accumulated in the bacterial cells. **C**) Gel-shift analysis of CsrA binding to RNA or ssDNA oligos equivalent to the RNA corresponding to pMO3 (**Methods**, **SI**), verifying binding of 1 or 2 CsrA molecules to single RNA and ssDNA oligos (first and second shift, respectively). In the first lane for comparison no CsrA is added. RNA or ssDNA was applied at 5 nM. **D**) Dissociation constants ($K_d$) for the binding of CsrA to various ssDNA oligos (**SI**). CsrA1 = stronger CsrA binding, CsrA2 = weaker CsrA binding.

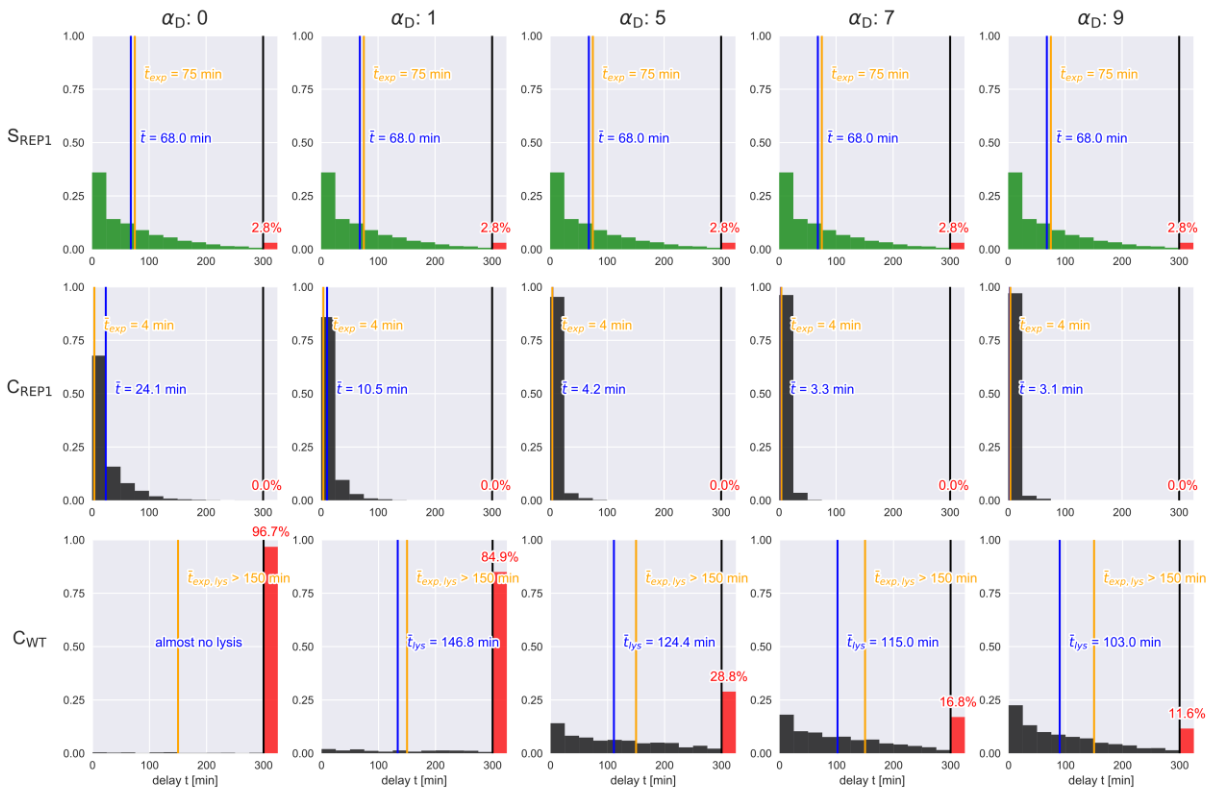


**Fig S6: *cea-cel* delay-time distributions and average *cea-cel* delay-times for different ssDNA production rates and strains.** The $S_{REP1}$ strain does not produce ssDNA, and is plotted (in green) only for the purpose of direct comparison with the $C_{REP1}$ strain. If no ssDNA is produced ($\alpha_D = 0$), we find that the $C_{REP1}$ strain shows a broader *cea-cel* delay-time distribution, compared to the cases with ssDNA production. The wild-type strain $C_{WT}$ does not lyse at all during the SOS signal for $\alpha_D = 0$. If we increase the ssDNA production rate, we find the experimentally observed behaviour that the $C_{REP1}$ strain shows very short *cea-cel* delays. In the wild-type strain, a certain threshold rate of ssDNA production is required to induce a significant level of lysis, emphasizing the importance of ssDNA for toxin release. Ensemble size: 2000 realisations.

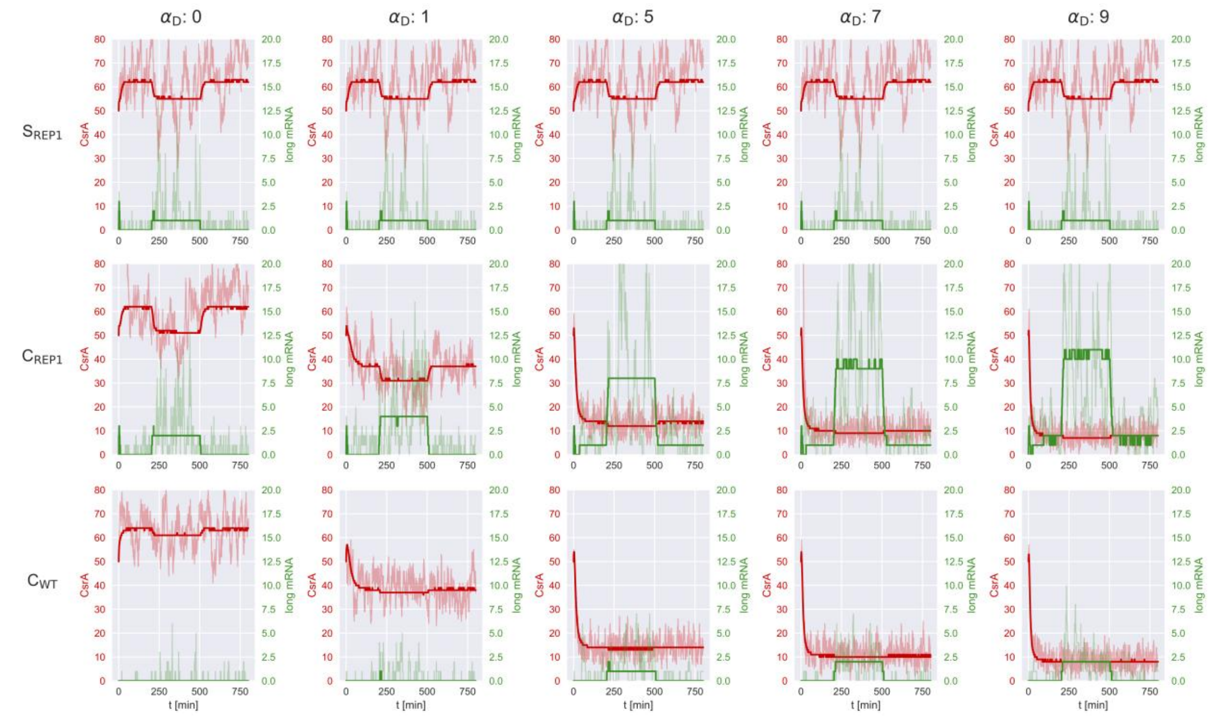


**Fig S7: Average of the time evolution of the CsrA and long mRNA abundance for different ssDNA production rates and strains.** Between t=200 and t=500, the system is subject to an SOS signal. In all cases, the SOS signal initiates a decrease in CsrA abundance from a previously stable level. This level is determined by the production, binding, and degradation rates of CsrA and its complex partners. As higher CsrA levels take longer and are also less likely to decrease to zero, they also directly affect the duration of the average *cea-cel* delay-time. The three plots for $\alpha_D = 0$ also show a single trajectory of long mRNA and CsrA in light green and light red, respectively. Ensemble size: 2000 realisations.

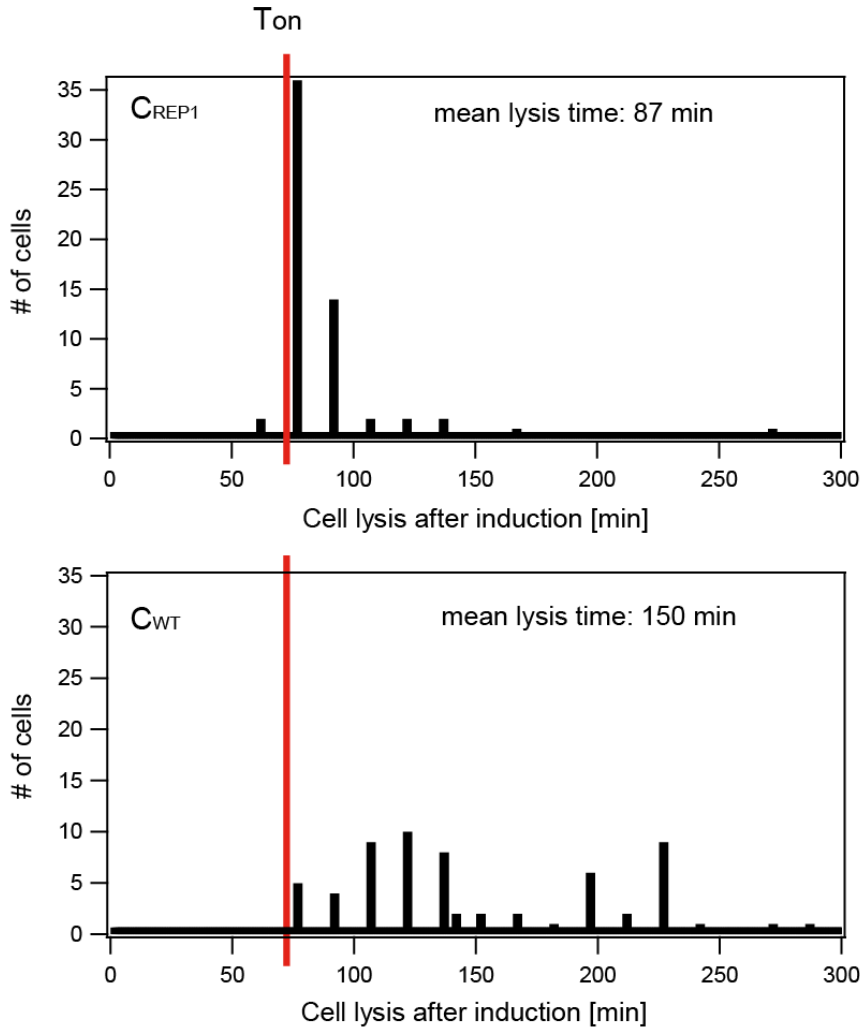


**Fig S8: Cell lysis after induction with 0.25 µg/ml MitC**. $C_{REP1}$ lyses on average 87 (± 3.9) min after induction with MitC, $C_{WT}$ lyses considerably later at 150 (± 6.9) min. For $C_{REP1}$, mean cell lysis nearly coincides with the $T_{ONcea}$ at 69.71 ± 0.77 min(7) (red line). This interval between $T_{ONcea}$ constitutes the delay between the SOS signal (MitC induction) and the start of *cea* gene expression. In our theoretical model, this initial delay is very short, as the system here switches directly from the pre-SOS signal 'OFF' state into the post-SOS signal 'ON' state. Hence, the red line also depicts the time-point of this switch (0 min in **Fig 4**).

## Supplementary References (experimental)


1. Morales M, Attai H, Troy K, Bermudes D. Accumulation of single-stranded DNA in Escherichia coli carrying the colicin plasmid pColE3-CA38. Plasmid. 2015;77:7-16. Epub 2014/12/03.
2. Khan SA. Plasmid rolling-circle replication: highlights of two decades of research. Plasmid. 2005;53(2):126-36. Epub 2005/03/02.
3. Yagura M, Nishio SY, Kurozumi H, Wang CF, Itoh T. Anatomy of the replication origin of plasmid ColE2-P9. Journal of bacteriology. 2006;188(3):999-1010. Epub 2006/01/24.
4. Aoki K, Shinohara M, Itoh T. Distinct functions of the two specificity determinants in replication initiation of plasmids ColE2-P9 and ColE3-CA38. Journal of bacteriology. 2007;189(6):2392-400. Epub 2007/01/24.
5. del Solar G, Kramer G, Ballester S, Espinosa M. Replication of the promiscuous plasmid pLS1: a region encompassing the minus origin of replication is associated with stable plasmid inheritance. Mol Gen Genet. 1993;241(1-2):97-105. Epub 1993/10/01.
6. Sugiyama T, Itoh T. Control of ColE2 DNA replication: in vitro binding of the antisense RNA to the Rep mRNA. Nucleic acids research. 1993;21(25):5972-7. Epub 1993/12/25.
7. Mader A, von Bronk B, Ewald B, Kesel S, Schnetz K, Frey E, et al. Amount of colicin release in Escherichia coli is regulated by lysis gene expression of the colicin E2 operon. PLoS One. 2015;10(3):e0119124. Epub 2015/03/10.
8. del Solar G, Giraldo R, Ruiz-Echevarria MJ, Espinosa M, Diaz-Orejas R. Replication and control of circular bacterial plasmids. Microbiol Mol Biol Rev. 1998;62(2):434-64. Epub 1998/06/10.
9. Kerr B, Riley MA, Feldman MW, Bohannan BJ. Local dispersal promotes biodiversity in a real-life game of rock-paper-scissors. Nature. 2002;418(6894):171-4. Epub 2002/07/12.
10. Zuker M. Mfold web server for nucleic acid folding and hybridization prediction. Nucleic acids research. 2003;31(13):3406-15. Epub 2003/06/26.
